# Supplementary material for: Exploring Feature Importance and Explainability Towards Enhanced ML-Based DoS Detection in AI Systems
Source: arXiv:2411.03355 source file (2024-11-04)
Supplement: Supplementary file 1 [file appendix.tex]

\begin{figure*}[htbp]
    \centering
    \includegraphics[height=15cm, width=14cm]{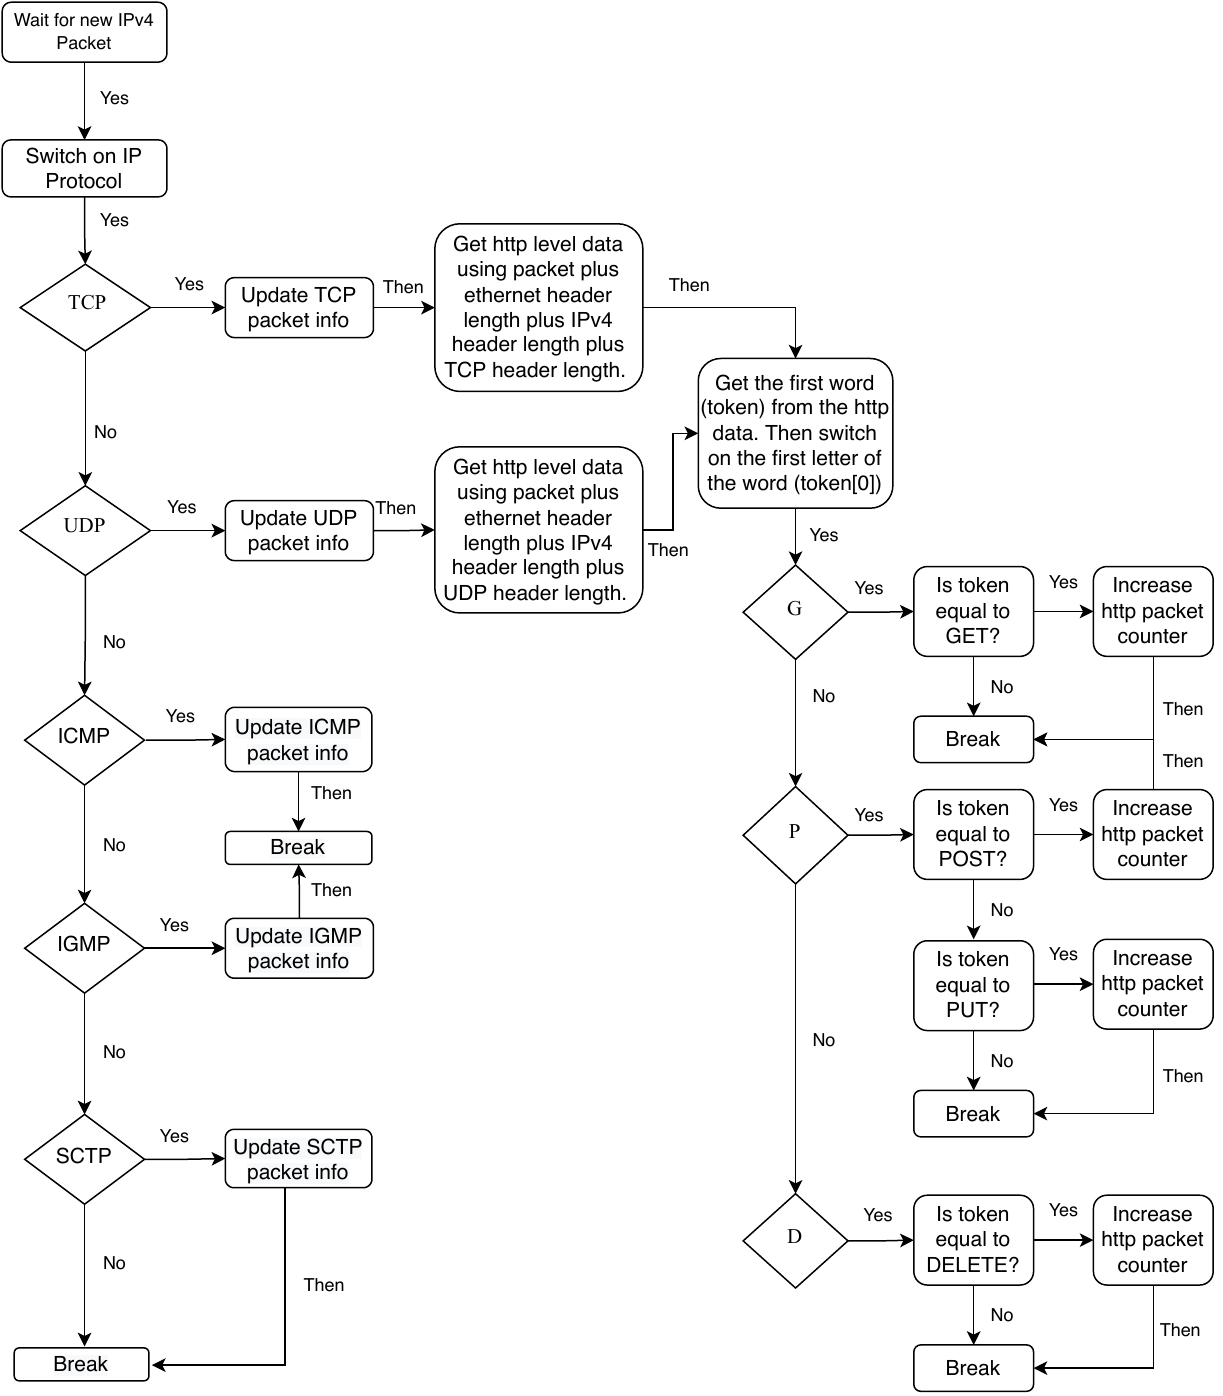}
    \caption{Flow chart for our HTTP layer data capture process.}
    \label{fig:http-capture}
\end{figure*}
